# Supplementary material for: Design choice and machine learning model performances
Source: arXiv:2201.10239 source file (2022-05-19)

# SUPPLEMENTAL MATERIAL

# Design choice and machine learning model performances

## 1. Test functions

Below you see the details of the test functions, including the ranges of the 6 input variables. Note that the outputs have been standardized and the range of the inputs has been converted to $[0,1]$. We also include a main effect plot for each test function, which provides a quick overview of the impact of each input on the output. Please, note that this is a rough approximation of the effect of the inputs on the output, and its sole objective is to give a quick view of the non-linearity present in the functions, but it cannot be considered an exhaustive representation of the behavior of $y$.

The main effect of a variable $x_i$ has been quantified as:

$$\overline{\text{me}}(x_i) \equiv \mathbb{E}\{y|x_i, \bar{x}_{-i}\}$$

**Borehole Function:**

$$y = 2\pi C(D - 760)/[\ln\left(\frac{B}{A}\right)(1 + \frac{2EC}{\ln\left(\frac{B}{A}\right)A^2F} + \frac{C}{89.6})]$$

| ID | Low level | High level |
|---|---|---|
| A | 0.05 | 0.15 |
| B | 100 | 50000 |
| C | 63070 | 115600 |
| D | 990 | 1110 |
| E | 1120 | 1680 |
| F | 1500 | 15000 |

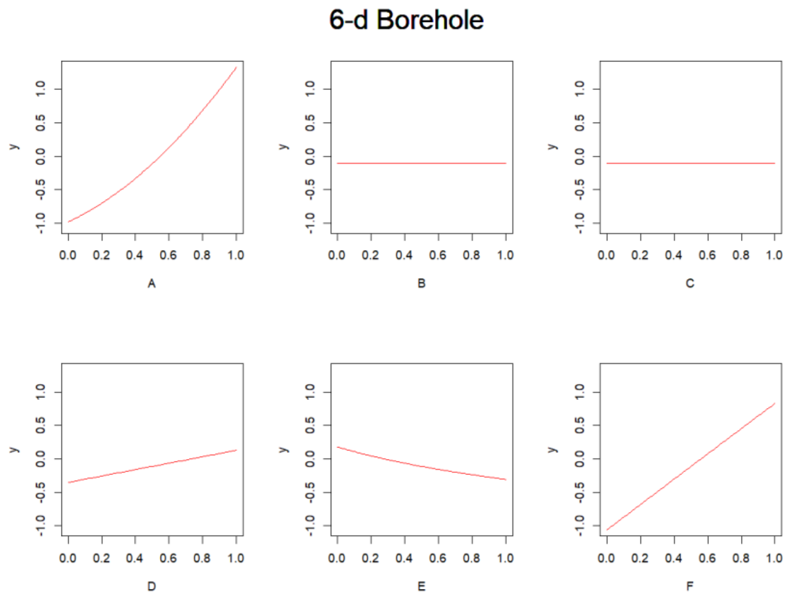

**OTL circuit Function:**

$y = \frac{(V_{b1}+0.74)F(E+9)}{F(E+9)+C} + \frac{11.35C}{F(E+9)+C} + \frac{0.74CF(E+9)}{(F(E+9)+C)D}$ , where $V_{b1} = \frac{12B}{A+B}$

| ID | Low level | High level |
|---|---|---|
| A | 50 | 150 |
| B | 25 | 70 |
| C | 0.5 | 3 |
| D | 1.2 | 2.5 |
| E | 0.25 | 1.2 |
| F | 50 | 300 |

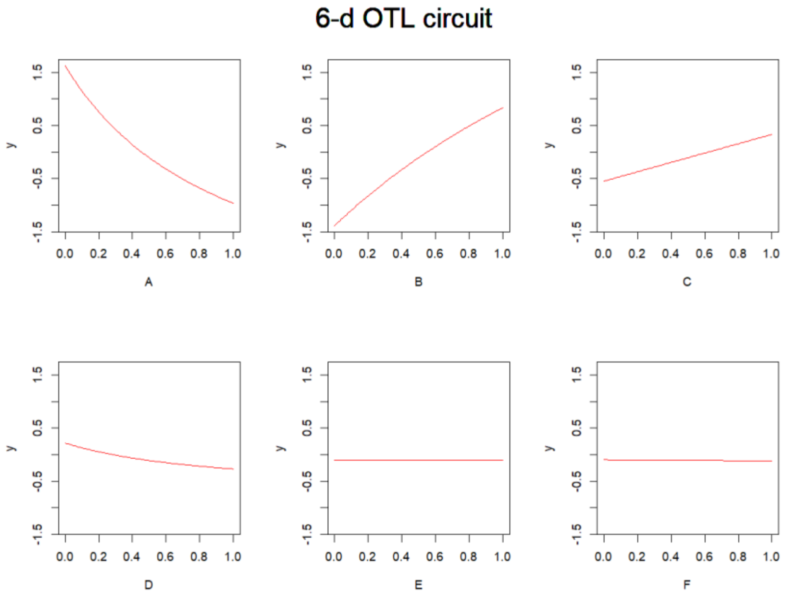

**Piston Function:**

$y = 2\pi\sqrt{\frac{A}{D+B^2*\frac{EC}{350}*F/V^2}} - W$, where $V = \frac{B}{2D}\left(\sqrt{4D*\frac{EC}{350}+W^2} - W\right)$, where $W = EB + 19.62A - \frac{DC}{B}$

| ID | Low level | High level |
|---|---|---|
| A | 30 | 60 |
| B | 0.005 | 0.02 |
| C | 0.002 | 0.01 |
| D | 1000 | 5000 |
| E | 90000 | 110000 |
| F | 290 | 296 |

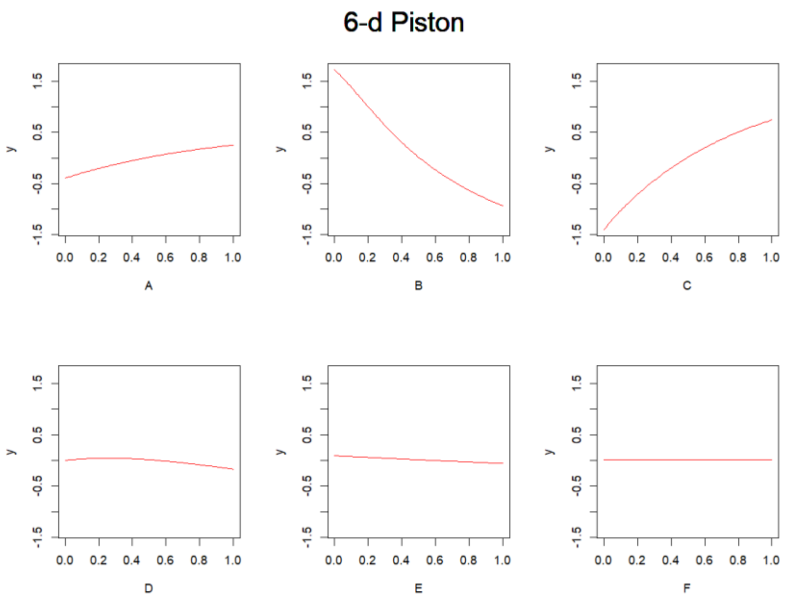

**Piston Mod Function:**

$y = 2\pi\sqrt{\frac{A}{D+B^2*\frac{EC}{350}*F/V^2}} - W$, where $V = \frac{B}{2D}\left(\sqrt{4D*\frac{EC}{350}+W^2} - W\right)$, where $W = EB + 19.62A - \frac{3DC}{B}$

| ID | Low level | High level |
|---|---|---|
| A | 30 | 60 |
| B | 0.005 | 0.02 |
| C | 0.002 | 0.01 |
| D | 1000 | 5000 |
| E | 90000 | 110000 |
| F | 290 | 296 |

6-d Piston Mod

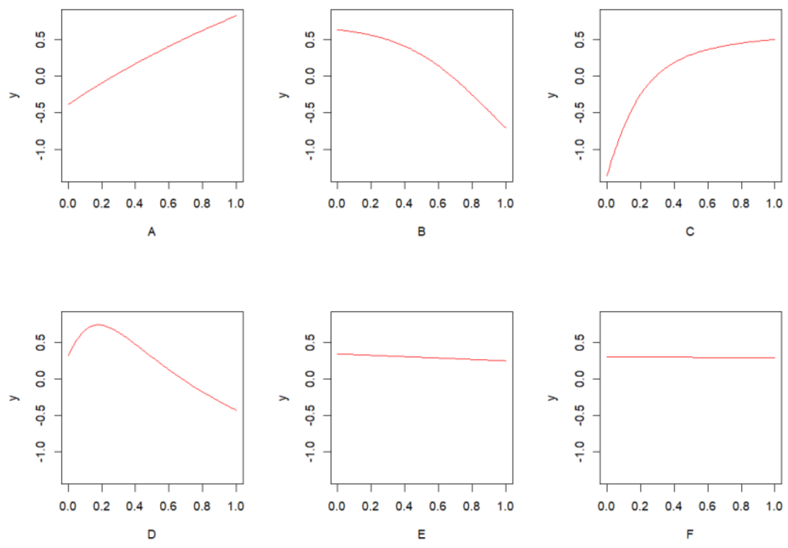

**Robot arm Function:**

$y = \sqrt{u^2 + v^2}$, where $u = \sum_{i=1}^{3} L_i \cos\left(\sum_{i=1}^{3} \theta_j\right)$, where $v = \sum_{i=1}^{3} L_i \sin\left(\sum_{i=1}^{3} \theta_j\right)$

| ID | Low level | High level |
|---|---|---|
| A ($\theta_1$) | 0 | $2\pi$ |
| B ($\theta_2$) | 0 | $2\pi$ |
| C ($\theta_3$) | 0 | $2\pi$ |
| D ($L_1$) | 0 | 1 |
| E ($L_2$) | 0 | 1 |
| F ($L_3$) | 0 | 1 |

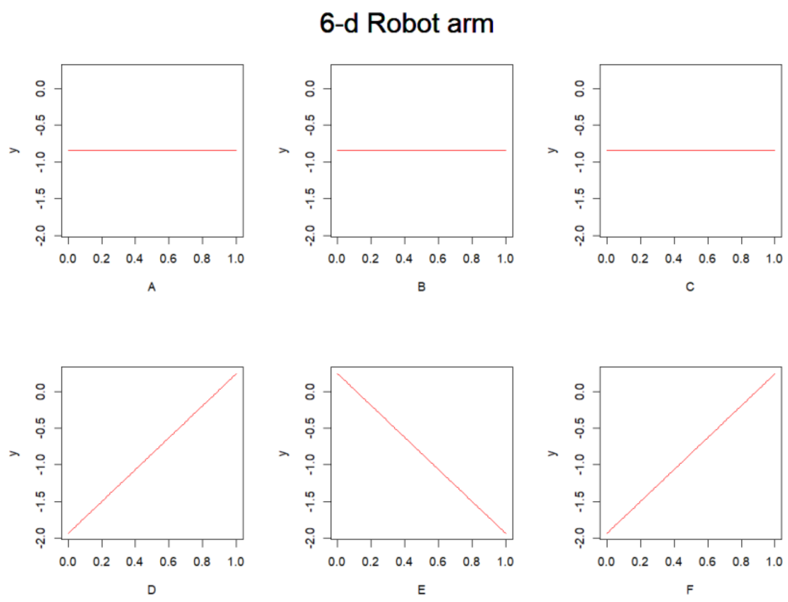

**Rosenbrock Function:**

$y = \sum_{i=1}^{d-1}[100(x_{i+1} - x_i^2)^2 + (x_i - 1)^2]$ , where $d = 6$

| ID | Low level | High level |
|---|---|---|
| A ($x_1$) | -5 | 10 |
| B ($x_2$) | -5 | 10 |
| C ($x_3$) | -5 | 10 |
| D ($x_4$) | -5 | 10 |
| E ($x_5$) | -5 | 10 |
| F ($x_6$) | -5 | 10 |

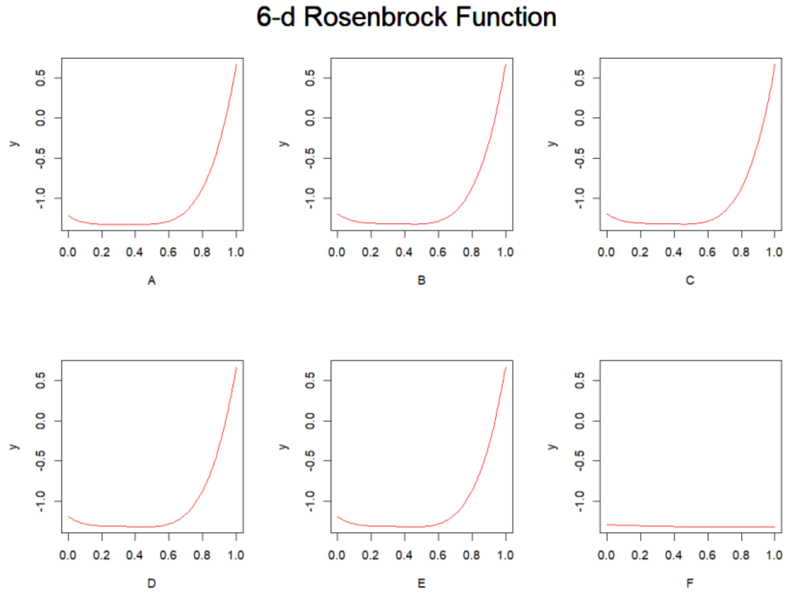

**Wing weight Function:**

$$y = 0.036A^{0.758}B^{0.0035}\left(\frac{8}{\cos^2(180\pi C)}\right)^{0.6} 30.5^{0.006}0.75^{0.04}\left(\frac{100D}{\cos(180\pi C)}\right)^{-0.3}(4E)^{0.49} + AF$$

| ID | Low level | High level |
|---|---|---|
| A | 150 | 200 |
| B | 220 | 300 |
| C | -10 | 10 |
| D | 0.08 | 0.18 |
| E | 1700 | 2500 |
| F | 0.025 | 0.08 |

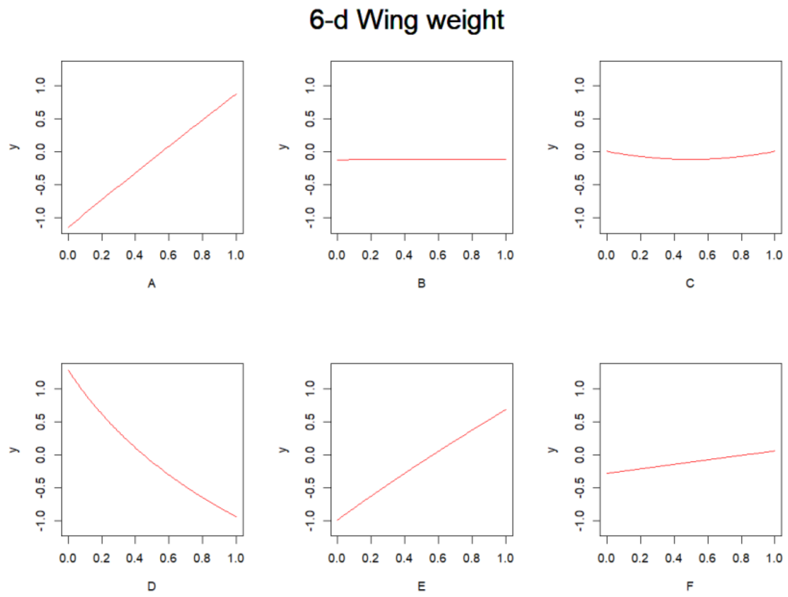

Supplement: Supplementary file 1 [file supplemental_material.pdf]
